# Supplementary material for: Integration of Preferences in Decomposition Multi-Objective Optimization
Source: arXiv:1701.05935 source file (2017-01-20)
Supplement: Supplementary file 1 [file appendix.tex]

% !tex root = main.tex

\appendices

\section{Choosing Pivot Point}
\label{app:pivotpoint}

In NUMS, the pivot point $\mathbf{w}^p$ is used to represent the ROI on the simplex $\Psi^m$. In this paper, we use the projection of the DM supplied aspiration level vector $\mathbf{z}^r$ onto $\Psi^m$ to serve this purpose. In theory, finding such projection is equivalent to solve the following minimization problem:
\begin{equation}
\mathbf{w}^p=\argmin_{\mathbf{w}\in\Psi^m}\|\mathbf{w}-\mathbf{z}^r\|
\label{eq:projection}
\end{equation}
As discussed in~\cite{ChenY11}, the solution of~(\ref{eq:projection}) is nontrivial and there does not have an explicit form. Here, we use the theorem developed in~\cite{ChenY11} to find such projection. \pref{alg:projection} gives the corresponding pseudo-code and interested readers are recommended to~\cite{ChenY11} for detailed mathematical deductions.
\begin{algorithm}

\KwIn{DM supplied aspiration level vector $\mathbf{z}^r$}
\KwOut{Pivot point $\mathbf{w}^p$ on $\Psi^m$}

Sort $\mathbf{z}^r$ in ascending order as $z^r_1\leq\cdots\leq z^r_m$;\\

\For{$i\leftarrow m-1$ \KwTo $1$}{
  $t_i\leftarrow\frac{\sum_{j=i+1}^mz^r_j-1}{m-i}$;\\
  \If{$t_i\geq z^r_i$}{
    $\hat{t}\leftarrow t_i$;\\
    \Return $\mathbf{w}^p\leftarrow[\mathbf{z}^r-\hat{t}]_+$
  }
}

$\hat{t}\leftarrow\frac{\sum_{j=1}^mz^r_j-1}{m}$;\\

\Return $\mathbf{w}^p\leftarrow[\mathbf{z}^r-\hat{t}]_+$

\caption{Projection of $\mathbf{z}^r\in\mathbb{R}^m$ onto the simplex $\Psi^m$} 
\label{alg:projection}
\end{algorithm}

\section{Proof of~\pref{theorem:eta}}
\label{app:eta}

\begin{figure}
\centering
\includegraphics[width=.9\linewidth]{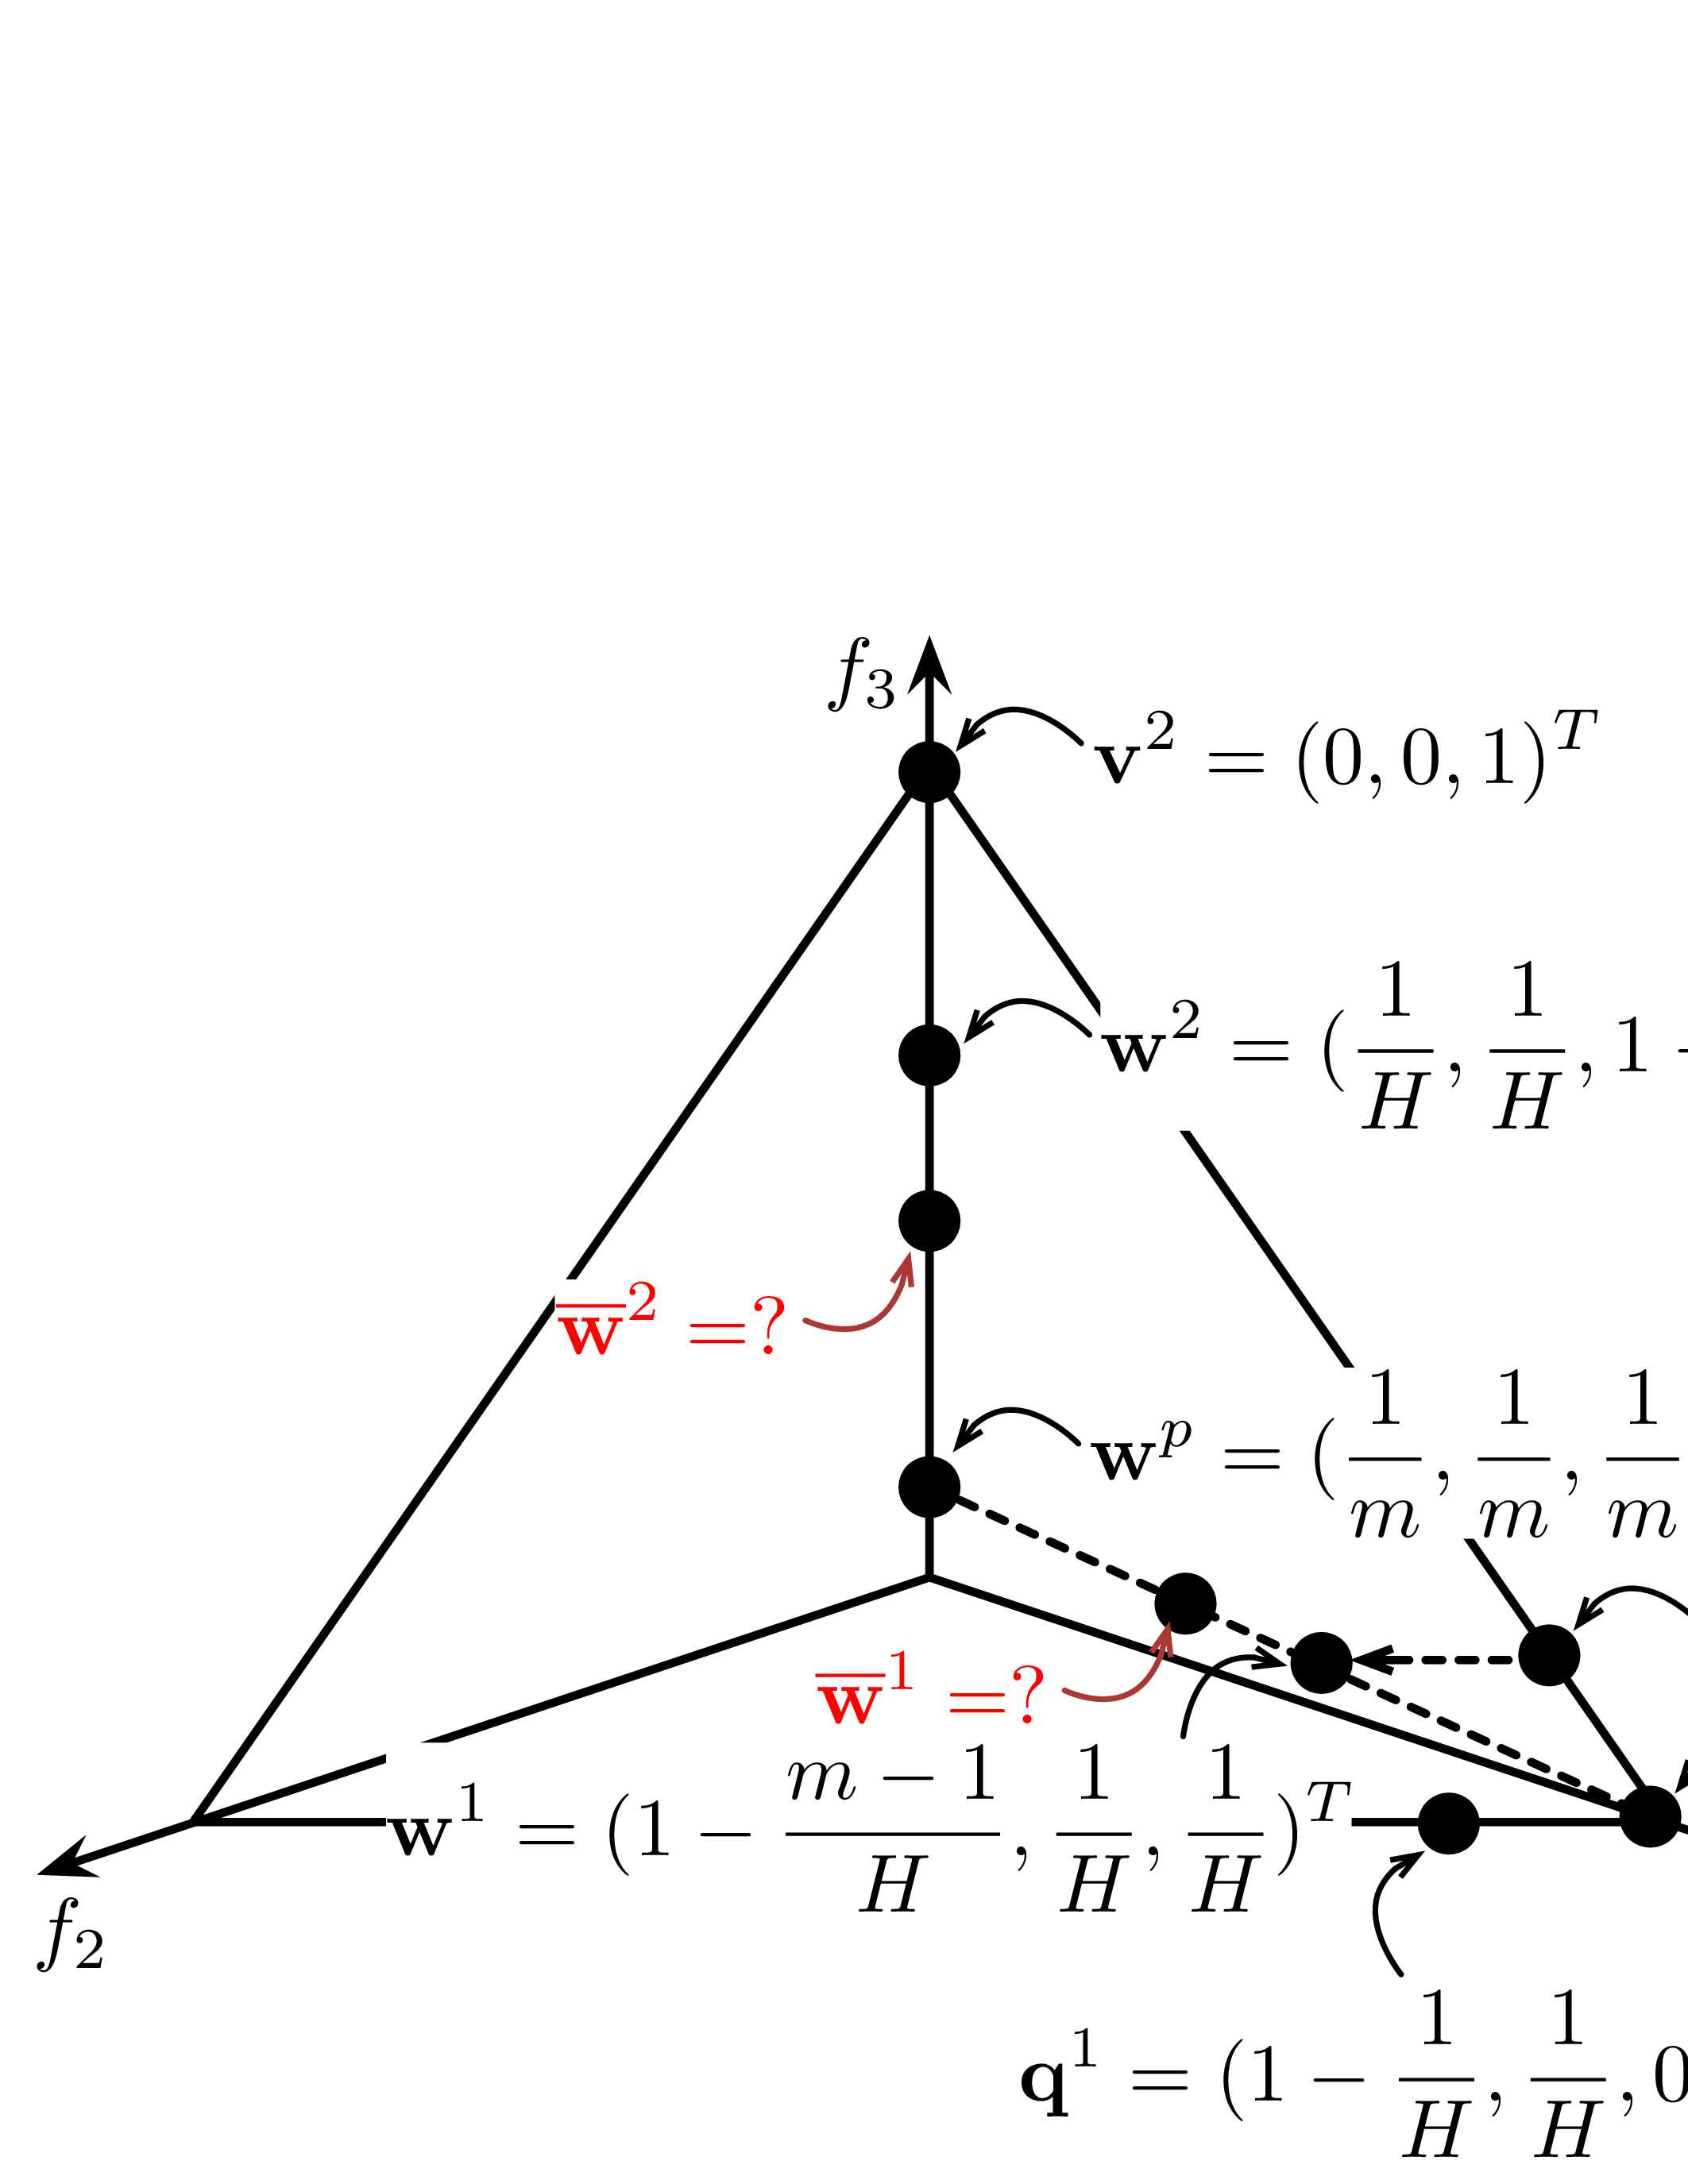}
\caption{Illustrative example for $\eta$ computation.}
\label{fig:etaexample}
\end{figure}

\begin{proof}
Let us use a specific example shown in~\pref{fig:etaexample} to prove this theorem. Suppose the reference points are originally generated by the Das and Dennis's method~\cite{NBI}. Therefore, reference points are distributed on an unit $m$-simplex. Let the centroid of this simplex, i.e., $\mathbf{w}^p=(\frac{1}{m},\cdots,\frac{1}{m})^T$, be the pivot point. Let us consider $\mathbf{v}^1=(1,0,0)^T$ and $\mathbf{v}^2=(0,0,1)^T$ as two vertices of an edge of this simplex. Obviously, the length of each edge of this simplex is the same, i.e., $\|\mathbf{v}^1-\mathbf{v}^2\|=\sqrt{2}$. Suppose $\mathbf{w}^1$ and $\mathbf{w}^2$ are two reference points inside this simplex and closest to $\mathbf{v}^1$ and $\mathbf{v}^2$. Since reference points are generated in a structured manner, we can use a geometric method to find the coordinates of $\mathbf{w}^1$ and $\mathbf{w}^2$. As shown in~\pref{fig:etaexample}, $\mathbf{q}^1$ and $\mathbf{q}^2$ are two reference points lying on the two edges and closest to $\mathbf{v}^1$. Obviously, $\mathbf{w}^1$ is a linear combination of $\mathbf{v}^1$, $\mathbf{q}^1$ and $\mathbf{q}^2$ as:
\begin{equation}
w_i^1=(q_i^2-v_i^1)+q_i^1
\end{equation}
where $i\in\{1,\cdots,m\}$. In summary, we can have $\mathbf{w}^1=(1-\frac{m-1}{H},\cdots,\frac{1}{H})^T$ and $\mathbf{w}^2=(\frac{1}{H},\cdots,1-\frac{m-1}{H})^T$. Based on our non-uniform mapping scheme, we have the new locations of $\mathbf{w}^1$ and $\mathbf{w}^2$ can be calculated as:
\begin{equation}
\mathbf{\overline{w}}^i=\mathbf{w}^p+t\times\mathbf{u}^i
\label{eq:use1}
\end{equation}
where $i\in\{1,2\}$, $\mathbf{u}^i=\frac{\mathbf{v}^i-\mathbf{w}^p}{\|\mathbf{v}^i-\mathbf{w}^p\|}$ and
\begin{equation}
t=d-d(\frac{d-D}{d})^{\frac{1}{\eta+1}}
\end{equation}
where $d=\|\mathbf{v^i-\mathbf{w}^p}\|$ and $D=\|\mathbf{w}^i-\mathbf{w}^p\|$. Let $q=\frac{d-D}{d}$, we have:
\begin{equation}
t=d(1-q^{\frac{1}{\eta+1}})
\label{eq:t}
\end{equation}
In order to have the extent of ROI become size of $\tau$ of the EF, we have the following equation:
\begin{equation}
\frac{\|\mathbf{\overline{w}}^1-\mathbf{\overline{w}}^2\|}{\|\mathbf{v}^1-\mathbf{v}^2\|}=\tau
\label{eq:rate1}
\end{equation}
Since $\|\mathbf{v}^1-\mathbf{v}^2\|=\sqrt{2}$, we have:
\begin{equation}
\|\mathbf{\overline{w}}^1-\mathbf{\overline{w}}^2\|=\sqrt{2}\tau
\label{eq:use2}
\end{equation}
Using~\pref{eq:use1} to substitute $\mathbf{\overline{w}}^1$ and $\mathbf{\overline{w}}^2$ in~\pref{eq:use2}, we have:
\begin{equation}
\|t\times(\mathbf{u}^1-\mathbf{u}^2)\|=\sqrt{2}\tau
\label{eq:use3}
\end{equation}
Using~\pref{eq:t} to substitute $t$ in~\pref{eq:use3}, we have:
\begin{equation}
d(1-q^{\frac{1}{\eta+1}})\times\|\mathbf{u}^1-\mathbf{u}^2\|=\sqrt{2}\tau
\label{eq:use4}
\end{equation}
By substitution, we have:
\begin{equation}
\begin{split}
(1-q^{\frac{1}{\eta+1}})\times\|\mathbf{v}^1-\mathbf{v}^2\|&=\sqrt{2}\tau\\
\implies q^{\frac{1}{\eta+1}}&=1-\tau\\
\implies \eta&=\frac{\log q}{\log(1-\tau)}-1
\end{split}
\end{equation}
Since the coordinates of $\mathbf{v}^1$, $\mathbf{w}^1$ and $\mathbf{w}^p$ are known, we have:
\begin{equation}
\begin{split}
d&=\sqrt{(1-\frac{1}{m})^2+(m-1)\frac{1}{m^2}}\\
&=\sqrt{1-\frac{1}{m}}
\end{split}
\label{eq:sd}
\end{equation}
and
\begin{equation}
\begin{split}
D&=\sqrt{(1-\frac{m-1}{H}-\frac{1}{m})^2+(m-1)(\frac{1}{m}-\frac{1}{H})^2}\\
&=\sqrt{1-\frac{1}{m}}(1-\frac{m}{H})\\
&=(1-\frac{m}{H})d
\end{split}
\label{eq:bd}
\end{equation}
Based on \pref{eq:sd} and \pref{eq:bd}, we have:
\begin{equation}
\begin{split}
q&=\frac{d-D}{d}\\
&=\frac{d-(1-\frac{m}{H})d}{d}\\
&=\frac{m}{H}
\end{split}
\label{eq:q}
\end{equation}
\end{proof}

\section{Proof of~\pref{corollary:boundseta}}
\label{app:boundseta}

\begin{proof}
As discussed in~\pref{sec:etasetting}, we should set $\eta>0$ in the NUMS. Thus, based on~\pref{theorem:eta}, we have:
\begin{equation}
\frac{\log\frac{m}{H}}{\log(1-\tau)}> 1\\
\end{equation}
Since $\frac{m}{H}<1$ and $1-\tau<1$, we have:
\begin{equation}
\begin{split}
\log\frac{m}{H}\leq\log(1-\tau)
\implies 0<\tau< 1-\frac{m}{H}
\end{split}
\end{equation}
\end{proof}

\section{Proof of~\pref{corollary:etaboundary}}
\label{app:etaboundary}

\begin{proof}
The proof of this corollary is similar to the \pref{theorem:eta}. Let us use \pref{fig:etaexample} for illustration again. As for the reference points $\mathbf{w}^1$ and $\mathbf{w}^2$, we should have the following relationship after the non-uniform mapping:
\begin{equation}
\frac{\|\mathbf{\overline{w}}^1-\mathbf{\overline{w}}^2\|}{\|\mathbf{w}^1-\mathbf{w}^2\|}=\tau
\label{eq:rate2}
\end{equation}
Since $\|\mathbf{w}^1-\mathbf{w}^2\|=\sqrt{2}(1-\frac{m}{H})$, we have:
\begin{equation}
\|\mathbf{\overline{w}}^1-\mathbf{\overline{w}}^2\|=\sqrt{2}(1-\frac{m}{H})\tau
\label{eq:use5}
\end{equation}
Using~\pref{eq:use1} to substitute $\mathbf{\overline{w}}^1$ and $\mathbf{\overline{w}}^2$ in~\pref{eq:use5}, we have:
\begin{equation}
\|t\times(\mathbf{u}^1-\mathbf{u}^2)\|=\sqrt{2}(1-\frac{m}{H})\tau
\label{eq:use6}
\end{equation}
Using~\pref{eq:t} to substitute $t$ in~\pref{eq:use6}, we have:
\begin{equation}
d(1-q^{\frac{1}{\eta+1}})\times\|\mathbf{u}^1-\mathbf{u}^2\|=\sqrt{2}(1-\frac{m}{H})\tau
\label{eq:use7}
\end{equation}

Since $\|\mathbf{v}^1-\mathbf{v}^2\|=\sqrt{2}$, by substitution, we have:
\begin{equation}
\begin{split}
1-q^{\frac{1}{\eta+1}}&=(1-\frac{m}{H})\tau\\
\implies \eta&=\frac{\log q}{\log[1-(1-\frac{m}{H})\tau]}-1
\end{split}
\label{eq:eta2}
\end{equation}
where $q=\frac{m}{H}$ according to \pref{eq:q}.
\end{proof}

\section{Proof of \pref{corollary:newbound}}
\label{app:newbound}

\begin{proof}
Since $\eta>0$, according to \pref{eq:eta2}, we have:
\begin{equation}
\frac{\log q}{\log[1-(1-\frac{m}{H})\tau]}>1
\end{equation}
Since $\frac{m}{H}<1$ and $1-(1-\frac{m}{H})\tau<1$, we have:
\begin{equation}
\log{\frac{m}{H}}<\log{[1-(1-\frac{m}{H})\tau]}\\
\implies 0<\tau<1
\end{equation}
\end{proof}
